# Supplementary material for: Entanglement Entropy at Large Central Charge
Source: arXiv:1303.6955 ancillary file (2013-03-27)
Supplement: Supplementary file 1 [file entanglement-at-large-c.nb.pdf]

**Supplemental Material for:**

# "Entanglement Entropy at Large Central Charge"

**by Thomas Hartman**

This *Mathematica* notebook contains implementations of the algorithms described in Appendix A of the paper, and a consistency check of the 5-interval accessory parameters in Figure 2 of the paper.

See the paper for references and further explanation.

*Tested in Mathematica version 8.0 for Mac OS X*

*Last updated:*

```
In[63]:= Date[][[1 ;; 3]]

Out[63]= {2013, 3, 16}
```

# Recursion relation for 4-pt conformal blocks

In[64]:=

```
Fq[c_, h_, hp_, x_, N_] := (16 q)^(hp + (1-c)/24) x^((c-1)/24 - h[[3]] - h[[4]]) (1 - x)^((c-1)/24 - h[[2]] - h[[3]])
    EllipticTheta[3, 0, q]^((c-1)/2 - 4 (h[[1]]+h[[2]]+h[[3]]+h[[4]])) * Hf[c, h, hp, q, N];
F[c_, h_, hp_, x_, N_] := (16 valq[x])^(hp + (1-c)/24) x^((c-1)/24 - h[[3]] - h[[4]]) (1 - x)^((c-1)/24 - h[[2]] - h[[3]])
    EllipticTheta[3, 0, valq[x]]^((c-1)/2 - 4 (h[[1]]+h[[2]]+h[[3]]+h[[4]])) * Hf[c, h, hp, valq[x], N];
Hf[c_, h_, H_, q_, N_] := 1 + Sum[((16 q)^(mn[[1]] mn[[2]]) R[mn, c, h])/(H - Hmn[mn, c]) Hf[c, h,
      Hmn[mn, c] + mn[[1]] mn[[2]], q, N - mn[[1]] mn[[2]]], {mn, mnpairsQ[N]}] /; N ≥ 0;
mnpairsQ[N_] := Select[Flatten[Table[{m, n}, {m, 1, N}, {n, 1, N}], 1],
    #[[1]] * #[[2]] ≤ N &];
αf[ϵ_, c_] := 1/Sqrt[24] (Sqrt[1 - c] + ϵ Sqrt[25 - c]);
Hmn[mn_, c_] := (c - 1)/24 + (mn[[1]] * αf[1, c] + mn[[2]] * αf[-1, c])^2/4;
valq[z_] := Exp[-π EllipticK[1 - z] / EllipticK[z]];
R[mn_, c_, h_] :=
   -1/2 Product[(zλ[h[[2]], c] + zλ[h[[1]], c] - zλpq[p, q, c]/2) (zλ[h[[2]], c] -
          zλ[h[[1]], c] - zλpq[p, q, c]/2) (zλ[h[[3]], c] + zλ[h[[4]], c] - zλpq[p, q, c]/2)
        (zλ[h[[3]], c] - zλ[h[[4]], c] - zλpq[p, q, c]/2),
       {p, -mn[[1]] + 1, mn[[1]] - 1, 2}, {q, -mn[[2]] + 1, mn[[2]] - 1, 2}] /
     Product[If[(aa == 0 && bb == 0) || (aa == mn[[1]] && bb == mn[[2]]), 1, zλpq[aa, bb, c]],
      {aa, -mn[[1]] + 1, mn[[1]]}, {bb, -mn[[2]] + 1, mn[[2]]}];
zλ[hi_, c_] := Sqrt[hi + (1 - c) / 24];
zλpq[p_, q_, c_] := αf[1, c] p + αf[-1, c] q;
(*
F[c, {h1, h2, h3, h4}, hp, x, N] is the conformal block
 with central charge c, external weights {h1, h2, h3, h4},
internal weight hp, and coordinate x, applying the recursion N times;

Fq[c, {h1, h2, h3, h4}, hp, x, N] is the same function,
but leaves the elliptic expansion parameter q = q[x] unevaluated.
*)
```

In[75]:=

```
(* Example: Standard series expansion *)

Fq[c, {h1, h2, h3, h4}, Δ, x, 2] /.
  q → Exp[-π EllipticK[1 - x] / EllipticK[x] + O[x]^2] // Simplify
```

Out[75]=

$$x^{-h3-h4+\Delta}\left(1-\frac{((h1-h2-\Delta)\ (h3-h4+\Delta))\ x}{2\ \Delta}+O[x]^{2}\right)$$

In[76]:=
```
(* Example: Plot it *)
testc = 22.0;
testh = testc / 12 * .7;
testΔ = testc / 12 * .456;
temp = Fq[testc, {h, h, h, h} /. h → testh, testΔ, x, 7];
Plot[temp /. q → valq[x], {x, 0, 1}]
```

Out[80]=

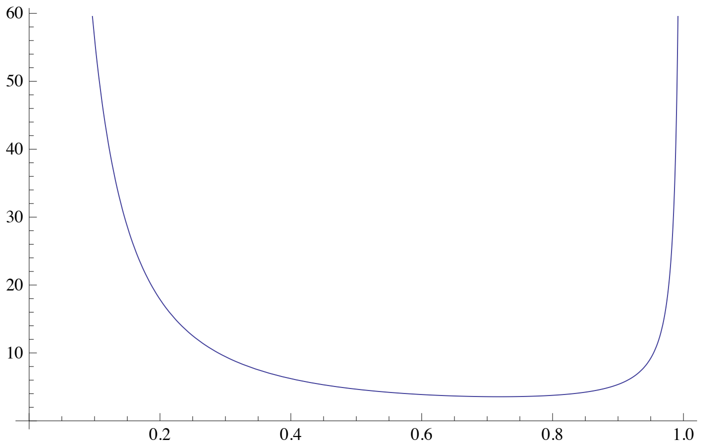


In[81]:=
```
(* Note that this is very accurate, even for x = 0.99;
check this by including a few more terms *)
(F[testc, {h, h, h, h} /. h → testh, testΔ, .99, 7] -
   F[testc, {h, h, h, h} /. h → testh, testΔ, .99, 9]) /
 F[testc, {h, h, h, h} /. h → testh, testΔ, .99, 7]
```

Out[81]= $-0.00107972 + 8.92773 \times 10^{-17}\, i$

# Numerical Monodromies

In[82]:=
```
monodromyMatrix[equation_, r_, center_: 0] :=
  Module[{icond, pareq, zfunc1, pareq1, ψ1, ψ2, MM, mm, a1, a2, a3},
   (* Arbitrary initial conditions *)
   icond = {a1 → .235, a2 → -.1948, a3 → .3245};
   (* differential equation parameterized on a circle *)
   pareq = equation /.
      {f[z] → f[t], f''[z] → (-u''[t])/(u'[t]^3) f'[t] + 1/(u'[t]^2) f''[t]} /. {z → z[t], u → z};
   zfunc1 = Function[center + r E^(I #)];
   pareq1 = pareq /. z → zfunc1;
   (* Solve the ODE on this contour  *)
   ψ1 =
    f /. NDSolve[{pareq1 == 0, f[0] == a1, (I f'[0])/(zfunc1'[0]) == a2} /. icond, f, {t, 0, 2 π}][[1]];
   (* Solve it again with different initial conditions *)
   ψ2 =
    f /. NDSolve[{pareq1 == 0, f[0] == a1, (I f'[0])/(zfunc1'[0]) == a3} /. icond, f, {t, 0, 2 π}][[1]];
   (* Solve for monodromy matrix *)
   MM = Array[mm, {2, 2}];
   MM /. Solve[MM.{ψ1[0], ψ2[0]} == {ψ1[2 π], ψ2[2 π]} &&
       MM.{ψ1'[0], ψ2'[0]} == {ψ1'[2 π], ψ2'[2 π]}, Flatten[MM]][[1]]
  ];
monodromyTrace[deq_, r_, center_: 0] := Tr[monodromyMatrix[deq, r, center]];
(* Find accessory parameter c2 that gives desired monodromy invariant *)
c2previous = .5;
(* here d = 6 h/c, with h the external weight *)
getC2[d_, x_, trM_] := Module[{deq, monoeq, c2, c3, c4 , meq2, c2val},
   deq = (d/(1 - z)^2 + d/z^2 + (2 d)/((1 - z) z) + d/(-x + z)^2 - (c2 (1 - x) x)/((1 - z) z (-x + z))) f[z] + f''[z];
   monoeq[c2val_] := Module[{testTrace},
     testTrace = monodromyTrace[deq /. {c2 → c2val}, x + .05,  0];
     Abs[Re[testTrace] - trM ] + Abs[Im[testTrace]]
    ];
   c2previous = c2 /. FindRoot[monoeq[c2],
      {c2, c2previous}, Evaluated → False, AccuracyGoal → 5, PrecisionGoal → 5]

  ];
```

In[86]:=
```
(*
Syntax:

monodromyMatrix[equation, r, center] computes the monodromy matrix,
in some arbitrary basis, for a second order differential
 equation around a circle of radius r centered at center;

monodromyTrace[equation, r, center] is similar but computes Tr M;

getC2[d,x,trM] finds the accessory parameter c2 such that the monodromy
  invariant of the 4pt equation with external weight h=c/6 d is trM;

*)
```

In[87]:=
```
(* Example: compute monodromies of the 4pt Fuchsian equation,
on a circle of radius 0.75 *)
```

In[88]:=
$$\text{eqn} = \left(\frac{d}{(1-z)^2} + \frac{d}{z^2} + \frac{2\,d}{(1-z)\,z} + \frac{d}{(-x+z)^2} - \frac{c2\,(1-x)\,x}{(1-z)\,z\,(-x+z)}\right) f[z] + f''[z];$$

```
params = {d → .35, c2 → .3, x → .6};

monodromyMatrix[eqn /. params, .75]
monodromyTrace[eqn /. params, .75]
```

Out[90]= {{0.335671 + 0.347877 i, -0.486118 + 1.04497 i}, {-0.158053 + 1.74073 i, -2.57156 - 0.347877 i}}

Out[91]= $-2.23589 - 3.11479 \times 10^{-8}\, i$

In[92]:=

```
(* Example: Find the accessory parameter c2,
with h = c/6*.31 and x=.1, which sets Tr M = 2 *)
getC2[.31, .1, 2]

(* c2previous sets the starting point for the minimization algorithm *)
c2previous = 2.5;
getC2[.31, .3, 2]
```

Out[93]= 6.1959

Out[95]= 2.03383

In[96]:=
```
(* Compare to the semiclassical conformal block *)
(* Note: run the recursion example first *)
testh = testc / 6 * .31;

temp = F[testc, {h, h, h, h} /. h → testh, 0.0, x, 5] /. q → valq[x];
```

$$D\left[\frac{\text{Log}[\text{temp}]}{(-\text{testc}/6)}, x\right] /.\ x \to .1$$

$$D\left[\frac{\text{Log}[\text{temp}]}{(-\text{testc}/6)}, x\right] /.\ x \to .3$$

Out[98]= $6.1925 + 1.18227 \times 10^{-19}\, i$

Out[99]= $2.03409 + 4.71139 \times 10^{-19}\, i$

# Example : Trivial monodromies for 5 disjoint intervals

In[100]:=
```
(*See figure 2 in the paper. We will confirm that c_i =
 12 α/(z_i - z_j) for small α imposes trivial monodromy
  around the cycles that pair the operators at z_i and z_j *)
```

In[101]:=
```
(* Number of external points *)
k = 10;
(* Stress tensor *)
T = Sum[d/(z - x[i])^2 - c[i]/(z - x[i]), {i, k}];
(* regularity of T at infinity *)
regularityConditions = Sum[{c[i], c[i] x[i] - d, c[i] x[i]^2 - 2 d x[i]}, {i, k}];
T = T /. Simplify[Solve[regularityConditions == 0, {c[1], c[k], c[k - 1]}][[1]]];
(* send 3 points to 0, 1, ∞ *)
T = (T /. {x[k] → 1 / ϵ, x[1] → 0, x[k - 1] → 1}) + O[ϵ] // Normal;
(* Final answer for T *)
T = Collect[T, z, Simplify];
(* Fuchsian equation *)
eqn = f''[z] + T f[z]
```

Out[107]=

$$f[z]\left(\frac{d}{(-1+z)^2}+\frac{d}{z^2}+\frac{d}{(z-x[2])^2}-\frac{c[2]}{z-x[2]}+\frac{d}{(z-x[3])^2}-\frac{c[3]}{z-x[3]}+\frac{d}{(z-x[4])^2}-\frac{c[4]}{z-x[4]}+\frac{d}{(z-x[5])^2}-\frac{c[5]}{z-x[5]}+\frac{d}{(z-x[6])^2}-\frac{c[6]}{z-x[6]}+\frac{d}{(z-x[7])^2}-\frac{c[7]}{z-x[7]}+\frac{d}{(z-x[8])^2}-\frac{c[8]}{z-x[8]}+\frac{1}{z}(8d+c[2]+c[3]+c[4]+c[5]+c[6]+c[7]+c[8]-c[2]x[2]-c[3]x[3]-c[4]x[4]-c[5]x[5]-c[6]x[6]-c[7]x[7]-c[8]x[8])+\frac{1}{-1+z}(-8d+c[2]x[2]+c[3]x[3]+c[4]x[4]+c[5]x[5]+c[6]x[6]+c[7]x[7]+c[8]x[8])\right)+f''[z]$$

In[108]:=
```
(* Choose a small external; we are only doing this to first order in α *)
α = .01;

(* Choose some insertion points *)
points = {x[1] → 0, x[2] → .1, x[3] → .22, x[4] → .28,
   x[5] → .47, x[6] → .61, x[7] → .67, x[8] → .91, x[9] → 1, x[10] → ∞};
(* Choose accessory parameter derived analytically at small H,
for the channel in figure 2 *)
pairs = {2, 1, 4, 3, 10, 7, 7, 6, 9, 8, 5};
accessories = Table[c[i] → 12 α / (x[i] - x[pairs[[i]]]), {i, 2, k - 2}] /. points
(* This is the equation with trivial monodromies;
accessory parameters are correct only to leading order in α,
so monodromies will not be exactly 1 *)
eqn2 = eqn /. d → 6 α /. points /. accessories
```

Out[111]= {c[2] → 1.2, c[3] → -2., c[4] → 2., c[5] → 0., c[6] → -2., c[7] → 2., c[8] → -1.33333}

Out[112]=

$$\left(0. + \frac{0.06}{(-1+z)^2} - \frac{1.33333}{-1+z} + \frac{0.06}{(-0.91+z)^2} + \frac{1.33333}{-0.91+z} + \frac{0.06}{(-0.67+z)^2} - \frac{2.}{-0.67+z} + \frac{0.06}{(-0.61+z)^2} + \frac{2.}{-0.61+z} + \frac{0.06}{(-0.47+z)^2} + \frac{0.06}{(-0.28+z)^2} - \frac{2.}{-0.28+z} + \frac{0.06}{(-0.22+z)^2} + \frac{2.}{-0.22+z} + \frac{0.06}{(-0.1+z)^2} - \frac{1.2}{-0.1+z} + \frac{0.06}{z^2} + \frac{1.2}{z}\right) f[z] + f''[z]$$

In[113]:=
```
(* Check that we have trivial monodromy as claimed around the paired cycles *)

MF = MatrixForm[Round[#, .001]] &;
(* 1,2 cycle *)
monodromyMatrix[eqn2, x[2] + .03 /. points, 0] // MF
(* 3,4 cycle *)
monodromyMatrix[eqn2, (x[4] - x[3])/2 + .03 /. points, (x[4] + x[3])/2 /. points] // MF
(* 6,7 cycle *)
monodromyMatrix[eqn2, (x[7] - x[6])/2 + .03 /. points, (x[7] + x[6])/2 /. points] // MF
(* 8,9 cycle *)
monodromyMatrix[eqn2, (x[9] - x[8])/2 + .03 /. points, (x[8] + x[9])/2 /. points] // MF
(* 5,10 cycle *)
monodromyMatrix[eqn2, x[4] + .03 /. points, 0] // MF
```

Out[114]//MatrixForm=

$$\begin{pmatrix} 1.003 & -0.003 - 0.001\,i \\ 0.003 - 0.001\,i & 0.997 \end{pmatrix}$$

Out[115]//MatrixForm=

$$\begin{pmatrix} 1. & 0. - 0.001\,i \\ 0. - 0.002\,i & 1. \end{pmatrix}$$

Out[116]//MatrixForm=

$$\begin{pmatrix} 0.994 - 0.001\,i & 0.006 - 0.002\,i \\ -0.006 - 0.003\,i & 1.006 + 0.001\,i \end{pmatrix}$$

Out[117]//MatrixForm=

$$\begin{pmatrix} 0.999 & 0.001 - 0.001\,i \\ -0.001 - 0.001\,i & 1.001 \end{pmatrix}$$

Out[118]//MatrixForm=

$$\begin{pmatrix} 1.003 & -0.003 - 0.001\,i \\ 0.003 - 0.002\,i & 0.997 \end{pmatrix}$$

In[119]:=
```
(* The monodromy around a non-
 trivial cycle should correspond to the twist operator running in the OPE *)
monodromyTrace[eqn2, x[5] + .03 /. points, 0]
(* This should be equal *)
traceM[δ_] := -2 Cos[π Sqrt[24] Sqrt[1 / 24 - δ]];
traceM[α]
```

Out[119]= $1.83991 - 4.28207 \times 10^{-7}\, i$

Out[121]= 1.83992
